# Supplementary material for: Transliteration of Judeo-Arabic Texts into Arabic Script Using Recurrent Neural Networks
Source: arXiv:2004.11405 source file (2020-10-21)
Supplement: Supplementary file 1 [file appendix.tex]

\chapter{Alignment Algorithm}
We used the following dynamic algorithm to align the Judeo-Arabic and Arabic texts. \\ \\
For:\\
$T_i^{[0,...,l_i-1]}=\left(t_i^{0},t_i^{1},...,t_i^{l_i-1}\right)$ -- word sequence with length $l_i$\\
$\epsilon$ -- the empty string \\ 
$\phi$ -- an empty sequence \\ \\
Define:\\
$\textit{AlignScore}\left( T_1^{[0,...,l_1-1]},T_2^{[0,...,l_2-1]}\right)$ 
\begin{align*}\label{eq}
=\begin{cases}
0, & \text{if } l_1=0 \wedge l_2=0  \\
\textit{AlignScore}\left(\phi,T_2^{[0,...,l_2-2]}\right) + \textit{editDist}\left(\epsilon,t_2^{l_2-1}\right), & \text{if } l_1=0\\
\textit{AlignScore}\left(T_1^{[0,...,l_1-2]},\phi\right) + \textit{editDist}\left(t_1^{l_1-1},\epsilon\right), & \text{if }l_2=0\\
\min \left\{\begin{array}{lr}
        \textit{AlignScore}\left(T_1^{[0,...,l_1-2]},T_2^{[0,...,l_1-2]}\right) + \textit{editDist}\left(t_1^{l_1-1},t_2^{l_2-1}\right),\\
        \textit{AlignScore}\left(T_1^{[0,...,l_1-2]},T_2^{[0,...,l_2-1]}\right) + \textit{editDist}\left(t_1^{l_1-1},\epsilon\right),\\
        \textit{AlignScore}\left(T_1^{[0,...,l_1-1]},T_2^{[0,...,l_1-2]}\right) + \textit{editDist}\left(\epsilon,t_2^{l_2-1}\right)
        \end{array}\right\}
 , & \text{otherwise}
\end{cases}
\end{align*}
\newpage
Remarks:
\begin{enumerate}
\item 
Memoizing at each stage what choice was made by the \textit{minimum} operator, enables to track back the desired alignment.
In order to implement this algorithm in a space non-consuming manner only the alignment scores of two levels of recursion where kept. This is sufficient since the \textit{minimum} operator operates only one level deep. Actual implementation was done by an iterative version.
\item The $\textit{editDist}$ maps both string to Judeo-Arabic according to the simple map from Table \ref{tab:simp_map}, before calculating the distance.
\item The $\textit{editDist}$ on the empty string is equivalent to the length of the other string.
\end{enumerate}

\chapter{Example Transliteration of Unseen Text}
\begin{figure}[ht]
    \centering
    \includegraphics[width=\textwidth]{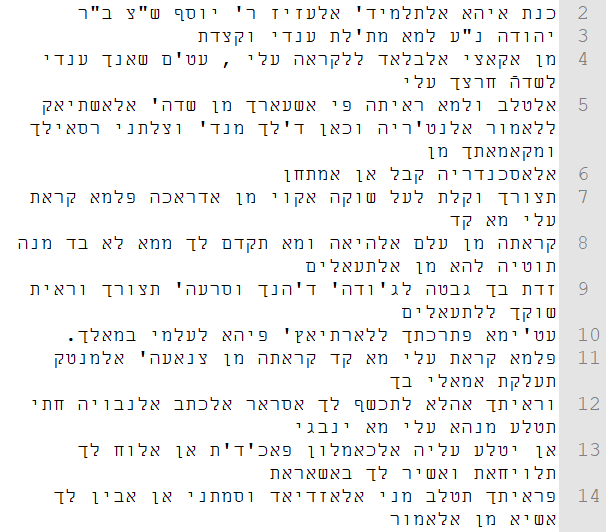}
    \caption{First page of {Maimonides}' \textit{The Guide for the Perplexed} in the original Judeo-Arabic orthography.}
    \label{fig:guide0}
\end{figure}
\begin{figure}[ht]
    \centering
    \includegraphics{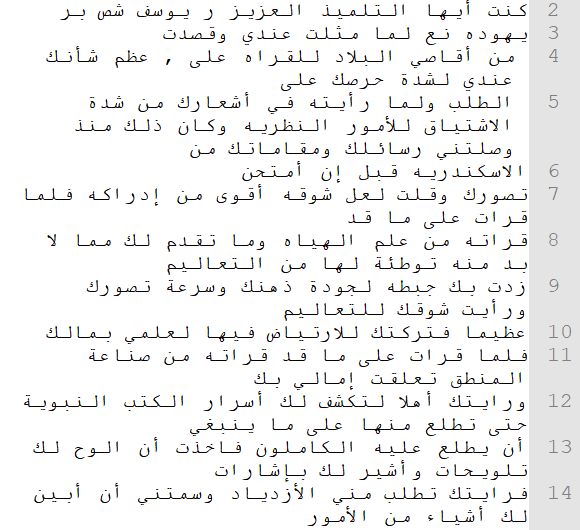}
    \caption{Our model transliteration of the first page of {Maimonides}' \textit{The Guide for the Perplexed} (final model trained with synthetic data).}
    \label{fig:guide}
\end{figure}
\begin{figure}
    \centering
    \includegraphics{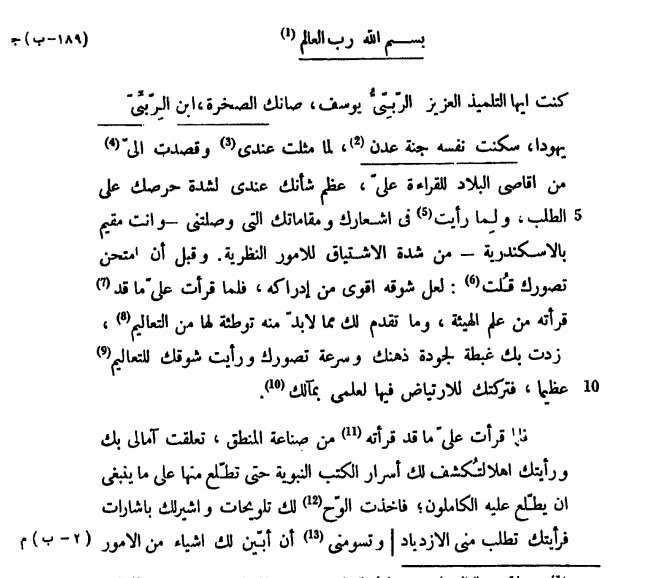}
    \caption{First page of {Maimonides}' \textit{The Guide for the Perplexed} as transliterated by {Hussein Attai}.}
    \label{fig:guide1}
\end{figure}
